# Supplementary material for: Principles of Visual Tokens for Efficient Video Understanding
Source: arXiv:2411.13626 source file (2025-03-23)
Supplement: Supplementary file 1 [file X_suppl.tex]

\clearpage
\setcounter{page}{1}
\setcounter{section}{0}
\maketitlesupplementary

\section{Additional Experimental Results}

Looking at the simplicity of LITE, one could think that learning to predict the \oracle is particularly easy and straightforward. After all, if an MLP can learn this, potentially a more sophisticated model should outperform it. 
This section describes the variants evaluated, giving additional insights and showcasing that token-selection is far from trivial. 

\myparagraph{Cleaning the \oracle training data.} Visualization suggests that the \oracle is somewhat noisy. Could we could clean the artifacts to improve the performance of the oracle? We explore several cleaning strategies:

\begin{itemize}
    \item Edges. Grad-CAM often produces noisy high activations at image boundaries. We decrease the values on edges to reduce boundary artifacts.
    \item Isolated peaks. The raw value of the \oracle often has isolated peaks, which can misrepresent the true important areas. 
    We remove small areas below a certain threshold. %
    \item Sharpening the distribution. The original distribution of the \oracle is often smooth. %
    We transform \oracle values %
    to amplify the differences between high and low values, making the distribution more concentrated around 0 or 1.
\end{itemize}

\myparagraph{Including global information.} The \model model assesses the value of a token based solely on the information of one token. This is a simplification of the way tokens are used, and overlooks qualities such as diversity of information, relationship, etc. 
We experimented with adding a global branch to \model, where instead of simply using the value of a token in isolation, we use several 3D convolutions to
acquire the nearby context information. Then, a self-attention operation is employed to capture long-range dependencies and model interactions between tokens, allowing the network to integrate global information effectively.

\myparagraph{Adding complexity to the selector.} A 3-layer MLP is a fairly simple model, and potentially we should be able to do better with a more sophisticated model. Adding layers or using other architectures can potentially lead to better results, even at the cost of an increased amount of computation. We experimented with several aspects. We used more layers (up to 5) to add capacity to the MLP. We also tried other architectures and replace the MLP with single or multiple transformer blocks.

It is remarkable to see in Table~\ref{tab:variants} that none of these variants significantly outperform the 3-layer MLP architecture. This points to a striking conclusion: the \oracle is extremely hard to predict, and the MLP achieves a balance between accuracy and avoiding overfitting.

\begin{table}
  \centering
  \small
  \begin{tabular}{lcc}
    \toprule
    Model  & Top-1 & Top-5 \\
    \midrule
    MLP selector & 65.03 & 88.52 \\
    Edges & 64.98 & 88.92 \\
    Isolated peaks & 64.83 & 88.67 \\
    Sharpen distribution & 64.80 & 87.98 \\
    Global branch & 65.10 & 88.55 \\
    \bottomrule
  \end{tabular}%
  \caption{Results of impact of different variants of data cleaning strategies and integration of global branch. Results are tested with 4K samples of the \ssv test set.
  } %
  \label{tab:variants}
\end{table}

\myparagraph{Adaptive budget.}
We test the adaptive budget results on the Kinetics-400 dataset, as detailed in Table ~\ref{tab:lite_adaptive_k400}. These results confirm consistency with our previous tests on the \ssv dataset. The LITE++ model is promising, enabling us to save nearly 30\% of \gflops compared to the LITE model, while maintaining the accuracy drop within 0.4.

\input{supplement/tables/adaptive_LITE++_k400}

\myparagraph{Adding complexity to the selector.} We test more sophisticated models as selectors for token selection, as shown in Table ~\ref{tab:complex_selector}. The experimental results indicate that using more complex architectures does not significantly improve accuracy but does substantially increase \gflops usage. Therefore, using simple 3-layer MLP is the optimal choice in balancing accuracy and \gflops.
\input{supplement/tables/complex_selector}

\myparagraph{Select tokens from different layers.}
Table~\ref{tab:select_from_diff_layers_ssv2} displays the results of our test involving token selection at various positions within the network. For instance, the experiment with block number of 0 indicates that token selection was performed before the first transformer block. Different block numbers correspond to token selection occurring before various transformer blocks. The experimental results reveal that token selection at the beginning of the network yields the best outcomes, whereas selection in the middle produces the worst results. Additionally, initiating token selection early in the process helps reduce \gflops significantly. Therefore, in the \model model, we position the selector before the first transformer block and conduct token selection at the outset.

\input{supplement/tables/select_from_different_layers}

\section{Additional Visualizations}

We present additional visualizations of token selection by our selector from the \ssv and Kinetics-400 datasets. These include the original RGB frames, along with the top 50\%, top 30\%, and top 10\% of tokens selected by our selector. The non-white areas indicate the tokens that have been selected.
Figures~\ref{fig:vis-k400-a} to~\ref{fig:vis-k400-d} show the visualization of the Kinetics-400 dataset, each labeled with its class. Figures~\ref{fig:vis-ssv2-a} to~\ref{fig:vis-ssv2-d} show the visualization of the \ssv dataset, each labeled with its class. 

\begin{figure*}
  \centering
    \includegraphics[width=0.95\linewidth]{supplement/figs/k400_310.png}
    \caption{Visualization of token selection by LITE in the Kinetics-400 dataset. Class label: ``skiing slalom".}
    \label{fig:vis-k400-a}
\end{figure*}
\begin{figure*}
  \centering
  \includegraphics[width=0.95\linewidth]{supplement/figs/k400_42.png}
    \caption{Visualization of token selection by LITE in the Kinetics-400 dataset. Class label: ``canoeing or kayaking".}
    \label{fig:vis-k400-b}
\end{figure*}
\begin{figure*}
  \centering  
  \includegraphics[width=0.95\linewidth]{supplement/figs/k400_274.png}
    \caption{Visualization of token selection by LITE in the Kinetics-400 dataset. Class label: ``riding scooter".}
    \label{fig:vis-k400-c}
\end{figure*}
\begin{figure*}
  \centering
  \includegraphics[width=0.95\linewidth]{supplement/figs/k400_217.png}
    \caption{Visualization of token selection by LITE in the Kinetics-400 dataset. Class label: ``playing accordion".}
    \label{fig:vis-k400-d}

\end{figure*}

\begin{figure*}
  \centering  
  \includegraphics[width=0.95\linewidth]{supplement/figs/ssv2_105.png}
    \caption{Visualization of token selection by LITE in the \ssv dataset. Class label: ``Putting something in front of something".}
    \label{fig:vis-ssv2-a}
\end{figure*}
\begin{figure*}
  \centering
  \includegraphics[width=0.95\linewidth]{supplement/figs/ssv2_84.png}
    \caption{Visualization of token selection by LITE in the \ssv dataset. Class label: ``Pretending to turn something upside down".}
    \label{fig:vis-ssv2-b}

\end{figure*}
\begin{figure*}
  \centering
  \includegraphics[width=0.95\linewidth]{supplement/figs/ssv2_164.png}
    \caption{Visualization of token selection by LITE in the \ssv dataset. Class label: ``Turning something upside down".}
    \label{fig:vis-ssv2-c}
\end{figure*}
\begin{figure*}
  \centering
  \includegraphics[width=0.95\linewidth]{supplement/figs/ssv2_107.png}
    \caption{Visualization of token selection by LITE in the \ssv dataset. Class label: ``Putting something next to something".}
    \label{fig:vis-ssv2-d}
\end{figure*}
